# Supplementary material for: Enhancing metallicity and basal plane reactivity of 2D materials via self-intercalation
Source: arXiv:2311.11131 source file (2023-11-18)
Supplement: Supplementary file 1 [file table1-raw.tex]

\begin{tabular}{lccccc}
\hline\hline
                 Parent ML  &  ic-fraction  &  $\Delta H_{f}$ (eV/atom)  &  $\Delta H_{hull}$ (eV/atom)  &  $E_{gap}$ (eV) & $\mu_{mag}$  \\
\hline
  \ce{Bi2Te3}  &    0.33     &     -0.18     &            45.2            &              0               &              0              \\
  \ce{Bi2Te3}  &    0.67     &     -0.14     &            76.1            &              0               &              0              \\
  \ce{Bi2Te3}  &      1      &     -0.11     &           102.8            &              0               &              0              \\
   \ce{CaI2}   &    0.33     &     -1.5      &            78.9            &             0.01             &              0              \\
  \ce{CrTe2}   &     0.5     &     -0.23     &            3.5             &              0               &            23.88            \\
  \ce{CrTe2}   &      1      &     -0.23     &            16.2            &              0               &            28.74            \\
   \ce{GaSe}   &    0.33     &     -0.53     &             51             &              0               &              0              \\
   \ce{GaSe}   &    0.67     &     -0.47     &            81.9            &              0               &              0              \\
   \ce{GaSe}   &      1      &     -0.45     &            87.2            &              0               &              0              \\
   \ce{GaS}($\alpha$)    &    0.33     &     -0.58     &            56.4            &              0               &              0              \\
   \ce{GaS}($\alpha$)    &    0.67     &     -0.53     &            84.7            &              0               &              0              \\
   \ce{GaS}($\alpha$)    &      1      &     -0.51     &            84.6            &              0               &              0              \\
   \ce{GaS}($\beta$)    &    0.33     &     -0.58     &            62.5            &              0               &              0              \\
   \ce{GaS}($\beta$)    &    0.67     &     -0.52     &            89.2            &              0               &              0              \\
   \ce{GaS}($\beta$)    &      1      &     -0.5      &            88.5            &              0               &              0              \\
   \ce{GaTe}   &    0.33     &     -0.32     &            40.3            &              0               &              0              \\
   \ce{GaTe}   &    0.67     &     -0.27     &             76             &              0               &              0              \\
   \ce{GaTe}   &      1      &     -0.23     &           105.2            &              0               &              0              \\
   \ce{GeS2}   &    0.75     &     -0.2      &           120.2            &             1.05             &              0              \\
   \ce{GeSe}   &    0.25     &     -0.15     &            68.6            &              0               &              0              \\
   \ce{GeSe}   &     0.5     &     -0.1      &           118.5            &              0               &              0              \\
  \ce{Hf3Te2}  &    0.25     &     -0.54     &            54.5            &              0               &              0              \\
  \ce{Hf3Te2}  &     0.5     &     -0.48     &            98.1            &              0               &              0              \\
 \ce{HfS2}(T)  &    0.33     &     -1.57     &           -39.2            &              0               &              0              \\
 \ce{HfS2}(T)  &    0.67     &     -1.52     &           -34.2            &              0               &              0              \\
 \ce{HfS2}(T)  &      1      &     -1.4      &            29.8            &              0               &              0              \\
 \ce{HfSe2}(T) &    0.33     &     -1.31     &            4.1             &              0               &              0              \\
 \ce{HfSe2}(T) &    0.67     &     -1.22     &            58.6            &              0               &              0              \\
 \ce{HfSe2}(T) &      1      &     -1.14     &           111.7            &              0               &              0              \\
 \ce{HfTe2}(T) &    0.33     &     -0.8      &            -2.1            &              0               &              0              \\
 \ce{HfTe2}(T) &    0.67     &     -0.73     &            45.7            &              0               &              0              \\
 \ce{HfTe2}(T) &      1      &     -0.66     &            95.7            &              0               &              0              \\
   \ce{InSe}   &    0.33     &     -0.49     &             24             &              0               &              0              \\
   \ce{InSe}   &    0.67     &     -0.44     &            51.9            &              0               &              0              \\
   \ce{InSe}   &      1      &     -0.42     &            52.8            &              0               &              0              \\
 \ce{MoS2}(H)  &    0.33     &     -0.75     &           118.3            &              0               &              0              \\
 \ce{MoS2}(H)  &    0.67     &     -0.68     &           146.9            &              0               &              0              \\
 \ce{MoS2}(H)  &      1      &     -0.62     &           169.1            &              0               &              0              \\
 \ce{MoSe2}(H) &    0.33     &     -0.51     &           158.3            &              0               &              0              \\
 \ce{MoTe2}(H) &    0.33     &     -0.11     &           189.9            &             0.02             &              0              \\
 \ce{NbS2}(H)  &    0.33     &     -1.17     &           -51.6            &              0               &              0              \\
 \ce{NbS2}(H)  &    0.67     &     -1.17     &           -12.1            &              0               &              0              \\
 \ce{NbS2}(H)  &      1      &     -1.13     &            55.5            &              0               &              0              \\
 \ce{NbS2}(T)  &    0.33     &     -1.1      &            23.6            &              0               &              0              \\
 \ce{NbS2}(T)  &    0.67     &     -1.05     &            103             &              0               &              0              \\
 \ce{NbSe2}(H) &    0.33     &     -0.9      &           -10.3            &              0               &              0              \\
 \ce{NbSe2}(H) &    0.67     &     -0.88     &            22.7            &              0               &              0              \\
 \ce{NbSe2}(H) &      1      &     -0.82     &            96.4            &              0               &              0              \\
\hline
\end{tabular}
