# Supplementary material for: Enhancing metallicity and basal plane reactivity of 2D materials via self-intercalation
Source: arXiv:2311.11131 source file (2023-11-18)
Supplement: Supplementary file 4 [file table2.tex]

\resizebox{0.67\textwidth}{!}{\begin{tabular}{lccccc}
\hline \hline
                Parent ML  &  ic-fraction  &  $\Delta H$ (eV/atom)  &  $\Delta H_{\mathrm{hull}}$ (meV/atom)  &  $E_{\mathrm{gap}}$ (eV) & $\mu_{\mathrm{mag}}$  \\
\hline
\rowcolor{Gray}
 \ce{NbSe2}(T) &    0.33     &     -0.85     &            41.8            &              0               &              0              \\
\rowcolor{Gray}
               &    0.67     &     -0.8      &           103.8            &              0               &              0              \\
\rowcolor{Gray}
               &      1      &     -0.75     &           161.9            &              0               &              0              \\
 \ce{NbTe2}(T) &    0.33     &     -0.4      &            68.8            &              0               &              0              \\
               &    0.67     &     -0.36     &           116.4            &              0               &              0              \\
               &      1      &     -0.31     &            176             &              0               &              0              \\
\rowcolor{Gray}
   \ce{PdS2}   &    0.25     &     -0.27     &            30.5            &             0.75             &              0              \\
\rowcolor{Gray}
               &     0.5     &     -0.26     &            53.4            &             0.6              &              0              \\
\rowcolor{Gray}
               &    0.75     &     -0.24     &            77.1            &             0.66             &              0              \\
  \ce{PdSe2}   &    0.25     &     -0.28     &            13.1            &             0.79             &              0              \\
               &     0.5     &     -0.27     &            32.8            &             0.71             &              0              \\
               &    0.75     &     -0.25     &            51.2            &             0.65             &              0              \\
\rowcolor{Gray}
 \ce{SnS2}(T)  &    0.33     &     -0.38     &            35.5            &              0               &              0              \\
\rowcolor{Gray}
               &    0.67     &     -0.36     &            62.1            &             0.02             &              0              \\
\rowcolor{Gray}
               &      1      &     -0.37     &            64.2            &              0               &              0              \\
 \ce{SnSe2}(T) &    0.33     &     -0.36     &            9.8             &              0               &              0              \\
               &    0.67     &     -0.36     &            17.5            &              0               &              0              \\
               &      1      &     -0.38     &            16.8            &              0               &              0              \\
\rowcolor{Gray}
   \ce{SnTe}   &    0.25     &     -0.18     &            87.1            &              0               &              0              \\
\rowcolor{Gray}
               &     0.5     &     -0.14     &            117             &              0               &              0              \\
 \ce{TaS2}(H)  &    0.33     &     -1.13     &           -75.3            &              0               &              0              \\
               &    0.67     &     -1.09     &           -70.2            &              0               &              0              \\
               &      1      &     -1.01     &           -17.8            &              0               &              0              \\
\rowcolor{Gray}
 \ce{TaS2}(T)  &    0.33     &     -1.05     &            2.3             &              0               &              0              \\
\rowcolor{Gray}
               &    0.67     &     -0.99     &            31.4            &              0               &              0              \\
\rowcolor{Gray}
               &      1      &     -0.91     &            73.1            &              0               &              0              \\
 \ce{TaSe2}(T) &    0.33     &     -0.77     &            34.5            &              0               &              0              \\
               &    0.67     &     -0.66     &           105.4            &              0               &              0              \\
               &      1      &     -0.56     &           175.6            &              0               &              0              \\
\rowcolor{Gray}
 \ce{TiTe2}(T) &    0.33     &     -0.72     &            -6.1            &              0               &              0              \\
\rowcolor{Gray}
               &    0.67     &     -0.69     &            28.7            &              0               &              0              \\
\rowcolor{Gray}
               &      1      &     -0.65     &            74.1            &              0               &            4.97             \\
  \ce{VS2}(H)  &    0.33     &     -0.96     &            -26             &              0               &            1.51             \\
               &    0.67     &     -0.96     &            23.8            &              0               &              0              \\
\rowcolor{Gray}
   \ce{W2N3}   &    0.33     &     -0.32     &            -135            &              0               &              0              \\
\rowcolor{Gray}
               &    0.67     &     -0.31     &           -121.1           &              0               &              0              \\
\rowcolor{Gray}
               &      1      &     -0.2      &           -15.6            &              0               &              0              \\
 \ce{WSe2}(T') &    0.33     &     -0.41     &           172.7            &              0               &             2.1             \\
               &    0.25     &     0.03      &           165.8            &              0               &              0              \\
               &     0.5     &     0.02      &           146.8            &              0               &            2.46             \\
\rowcolor{Gray}
   \ce{ZrBr}   &    0.33     &     -0.81     &           187.2            &              0               &              0              \\
  \ce{ZrCl2}   &    0.25     &     -1.48     &           165.3            &              0               &            2.08             \\
               &    0.33     &     -1.14     &           135.4            &              0               &             2.2             \\
               &    0.67     &     -1.03     &           198.7            &              0               &              0              \\
\rowcolor{Gray}
 \ce{ZrSe2}(T) &    0.33     &     -1.38     &           -60.4            &              0               &              0              \\
\rowcolor{Gray}
               &    0.67     &     -1.35     &           -65.7            &              0               &              0              \\
\rowcolor{Gray}
               &      1      &     -1.3      &           -49.8            &              0               &              0              \\
\hline
\end{tabular}}
